# Supplementary material for: Bond-selective fragmentation of water molecules with intense, ultrafast, carrier envelope phase stabilized laser pulses
Source: arXiv:1307.7552 source file (2013-07-29)

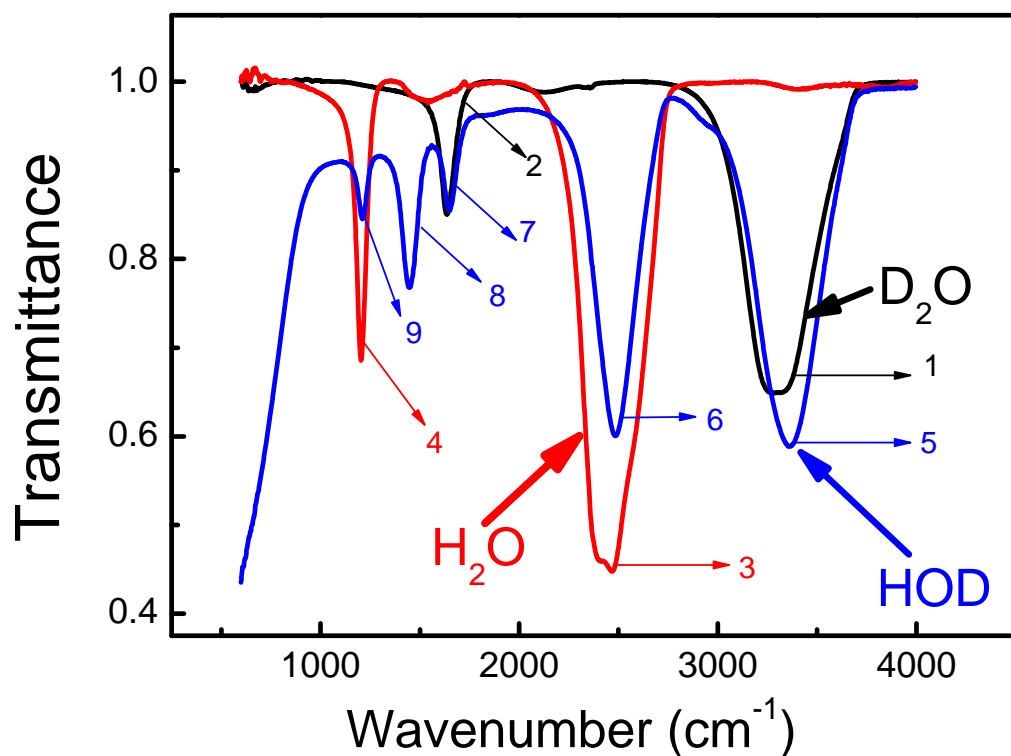

Absorption spectra measured from a mixture of H<sub>2</sub>O and D<sub>2</sub>O, showing vibrational peaks from these two molecules as well as from HOD. The individual peak numbers are correlated with vibrational features identified in the Table below.

| Peak # | Species          | Wavenumber (cm <sup>-1</sup> ) | Mode                  |
|--------|------------------|--------------------------------|-----------------------|
| 1      | H <sub>2</sub> O | 3277                           | Stretching            |
| 2      | H <sub>2</sub> O | 1635                           | Bending               |
| 3      | D <sub>2</sub> O | 2435                           | Stretching            |
| 4      | D <sub>2</sub> O | 1203                           | Bending               |
| 5      | HOD              | 3364                           | Stretching            |
| 6      | HOD              | 2485                           | Asymmetric Stretching |
| 7      | HOD              | 1651                           | Bending               |
| 8      | HOD              | 1445                           | Bending               |
| 9      | HOD              | 1210                           | Bending               |

Typical coincidence maps showing formation of ions pairs upon Coulomb explosion of  $\text{HOD}^{2+}$ ,  $\text{H}_2\text{O}^{2+}$ , and  $\text{D}_2\text{O}^{2+}$  at CEP values of 0 and  $\pi/2$ .

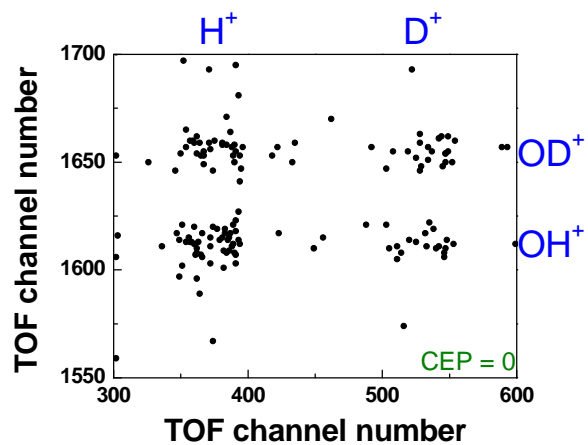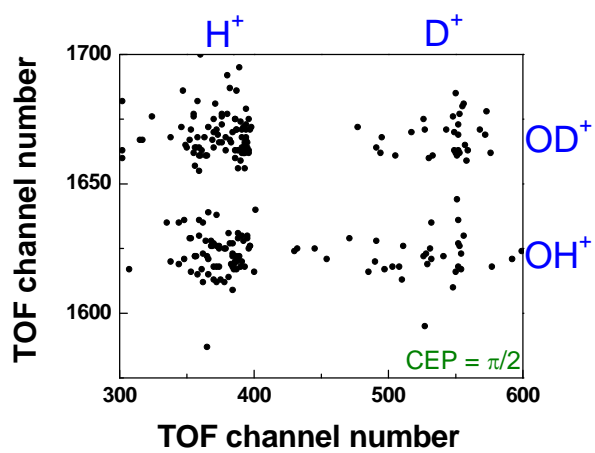

Supplement: Supplementary file 1 [file Supplemental_Material.pdf]
